# Supplementary material for: First principles study of hBN-AlN short-period superlattice heterostructures
Source: arXiv:1812.07188 source file (2018-12-18)
Supplement: Supplementary file 1 [file Suppl_Mat.pdf]

# Supplementary Material for
# "First principles study of hBN-AlN short-period superlattice heterostructures"

Catalin D. Spataru
*Sandia National Laboratories, Livermore, California 94551, USA*

Mary H. Crawford and Andrew A. Allerman
*Sandia National Laboratories, Albuquerque, New Mexico 87123, USA*

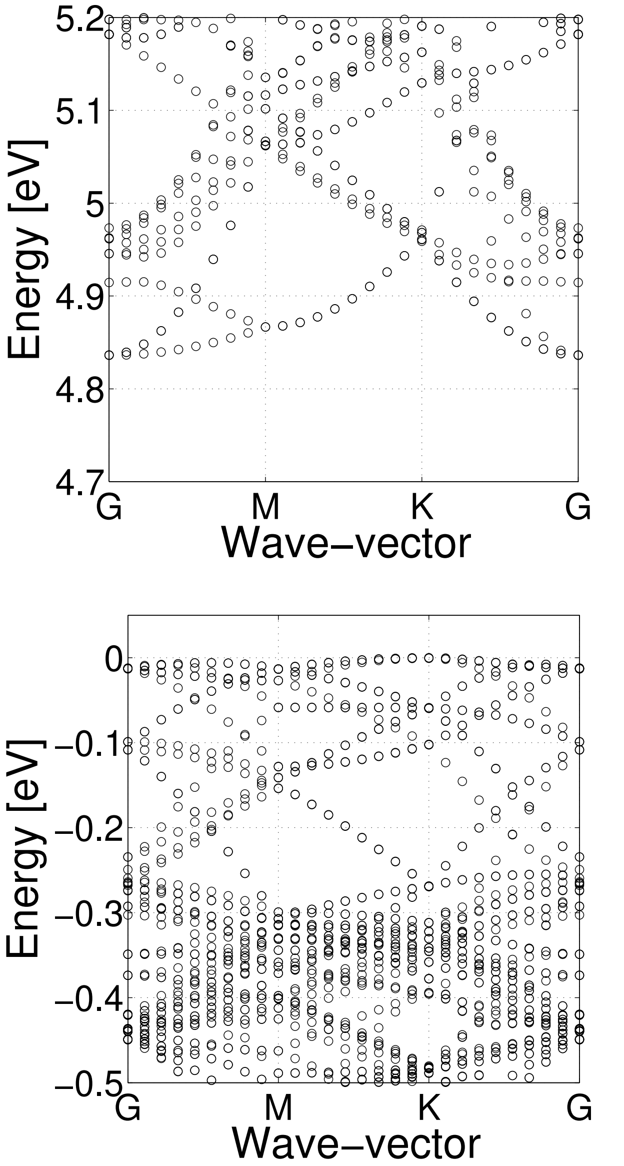


FIG. S1: Calculated electronic bandstructure of the $(hBN)_3(hAlN)_4$ SL calculated within hybrid DFT (HSE06) along several high symmetry directions in the Brillouin zone ($G$ stands for the $\Gamma$-point). a) electronic states near CBM, b) electronic states near VBM.

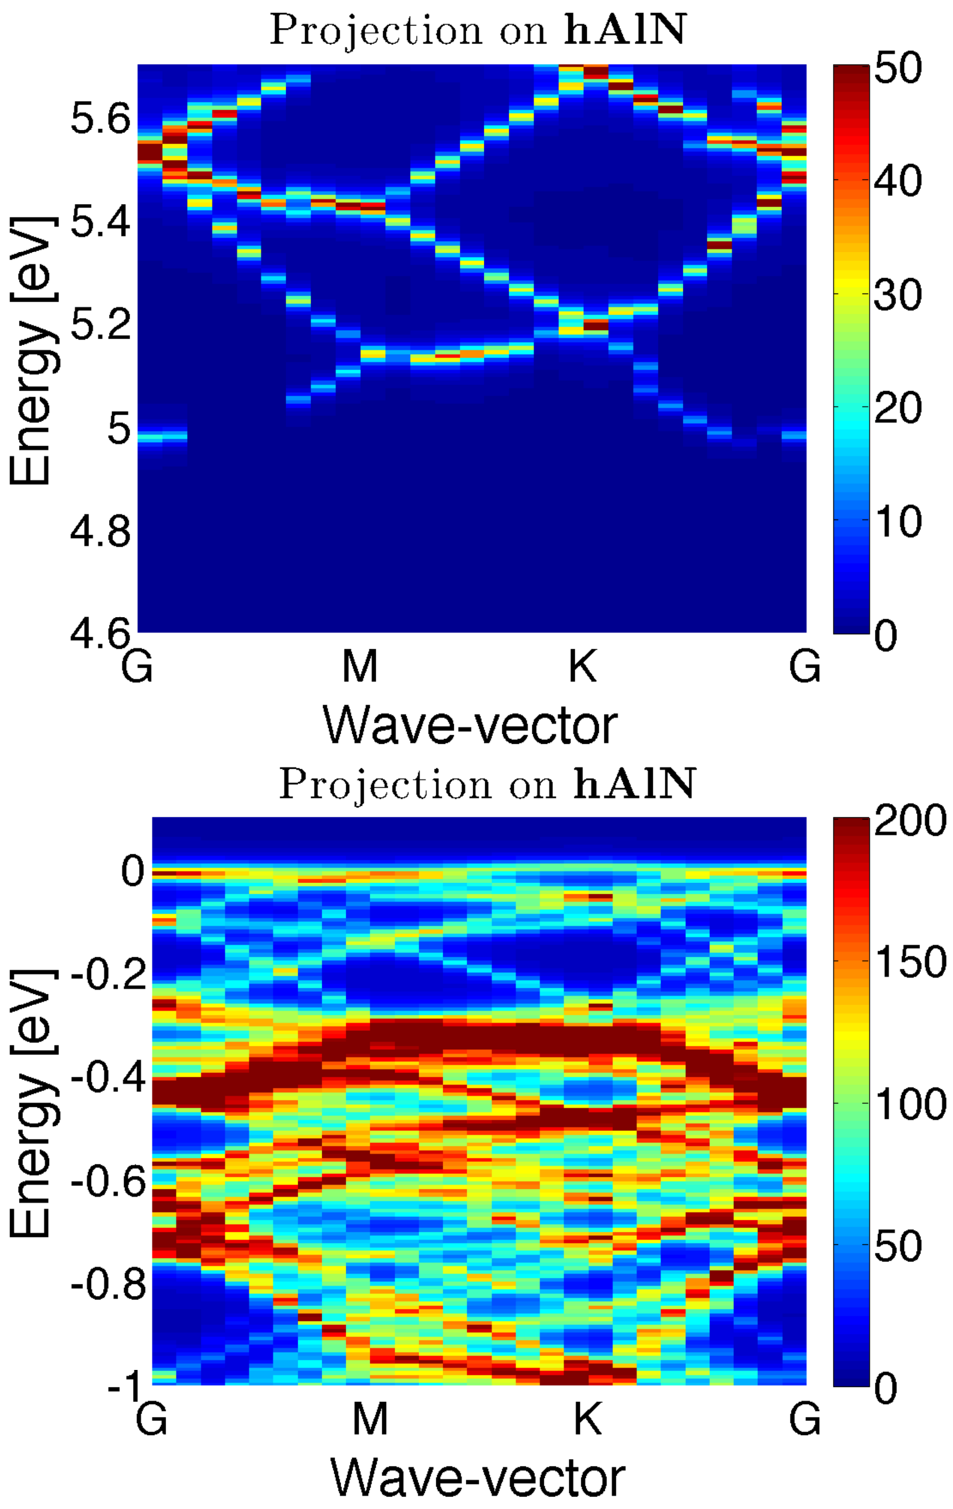


FIG. S2: Layer-projected electronic band-structure of the $(hBN)_3(hAlN)_4$ SL calculated within hybrid DFT (HSE06) with the color-map indicating the weight (arb. units) of electronic wavefunctions. a) states near CBM, b) states near VBM. Projection on the AlN layer.

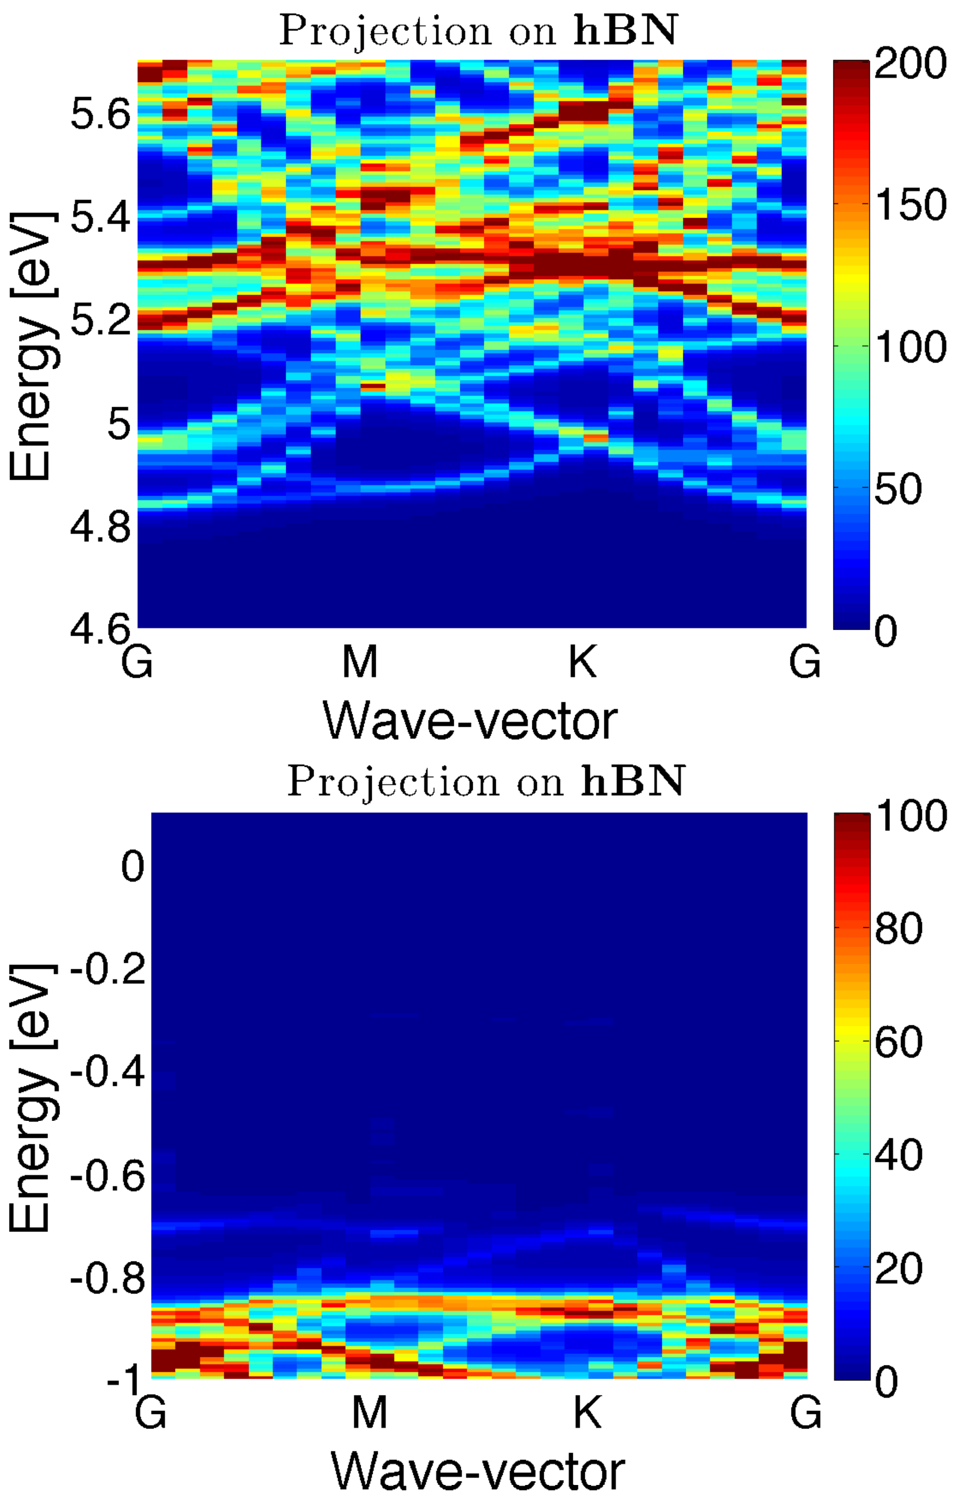


FIG. S3: Layer-projected electronic band-structure of the $(hBN)_3(hAlN)_4$ SL calculated within hybrid DFT (HSE06) with the color-map indicating the weight (arb. units) of electronic wavefunctions. a) states near CBM, b) states near VBM. Projection on the hBN layer.

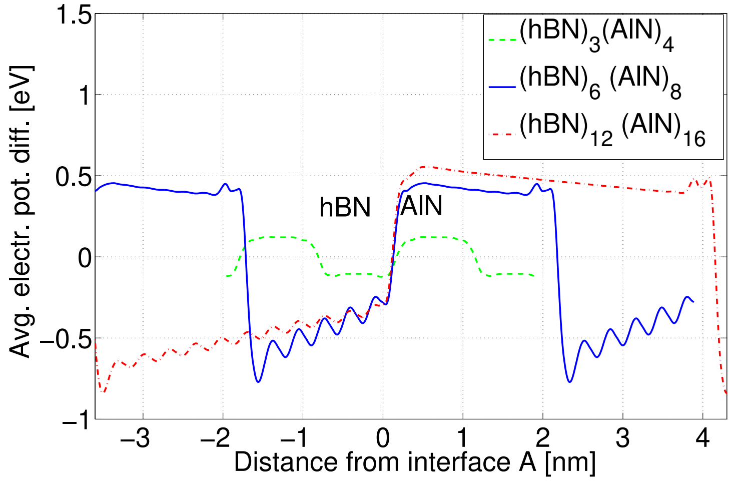


FIG. S4: Average electrostatic potential difference (between the SL and the sum of the isolated layers -the structure of an isolated layer is obtained by simply removing the atoms from the other layer in the SL) profile $V_{\rm diff}$ along [0001] for the $(hBN)_3(AlN)_4$, $(hBN)_6(AlN)_8$ and $(hBN)_{12}(AlN)_{16}$ SL obtained within hybrid-DFT (HSE06). $V_{\rm diff}$ captures the electronic charge redistribution upon joining the (relaxed) hBN and AlN layers. We note that at the interfaces between layers the change in $V_{\rm diff}$ has a different sign than the change in the macroscopic electrostatic potential shown in fig. 3 of the main text, reflecting the formation of charge-transfer interface dipoles that tend to partially compensate for the intrinsic difference between the average crystal potential in the two different compounds.

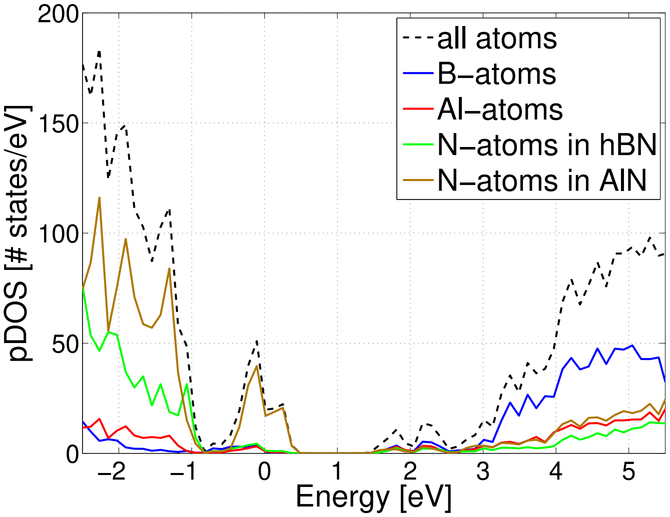


FIG. S5: Orbital projected DOS (pDOS) for $(hBN)_{12}(AlN)_{16}$. Dashed line: all atomic orbitals are included. Solid lines represent projection on: B-atoms (in blue), Al-atoms (in red), N-atoms in the hBN layer (in green) and N-atoms in the AlN layer (in brown). Results obtained within hybrid-DFT (HSE06).

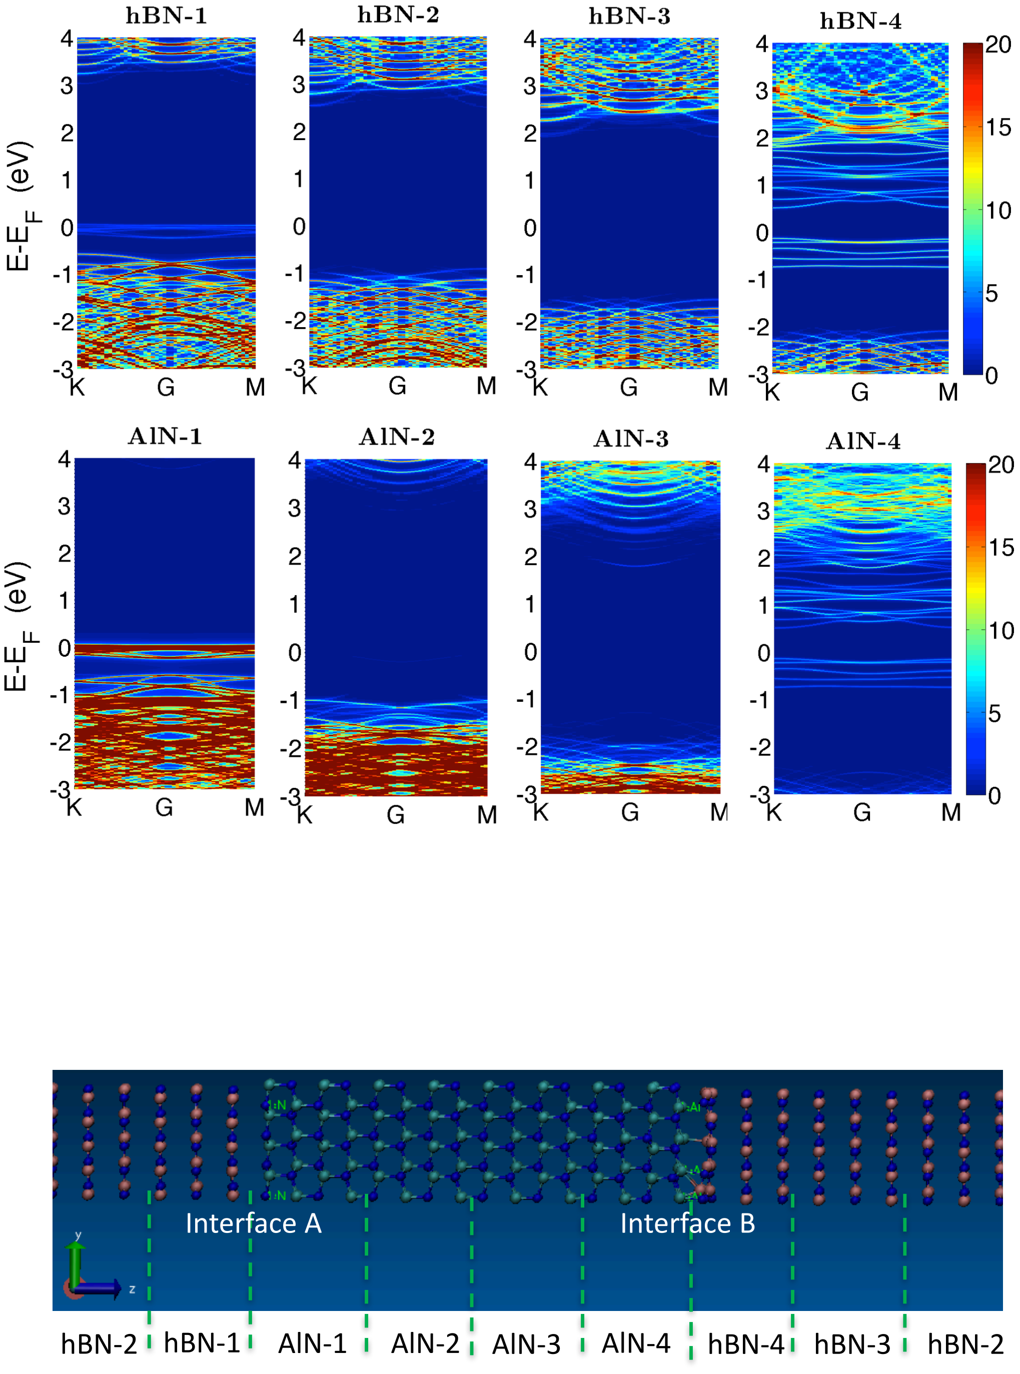


FIG. S6: a) Projected electronic band-structure of the $(hBN)_{12}(hAlN)_{16}$ SL calculated within LDA with the color-map indicating the weight (arb. units) of electronic wavefunctions on hBN (upper panels) or AlN (lower panels) sub-layers. b) Side view of the $(hBN)_{12}(hAlN)_{16}$ supercell structure. Green dashed lines indicate the sub-layers used for projection at a).

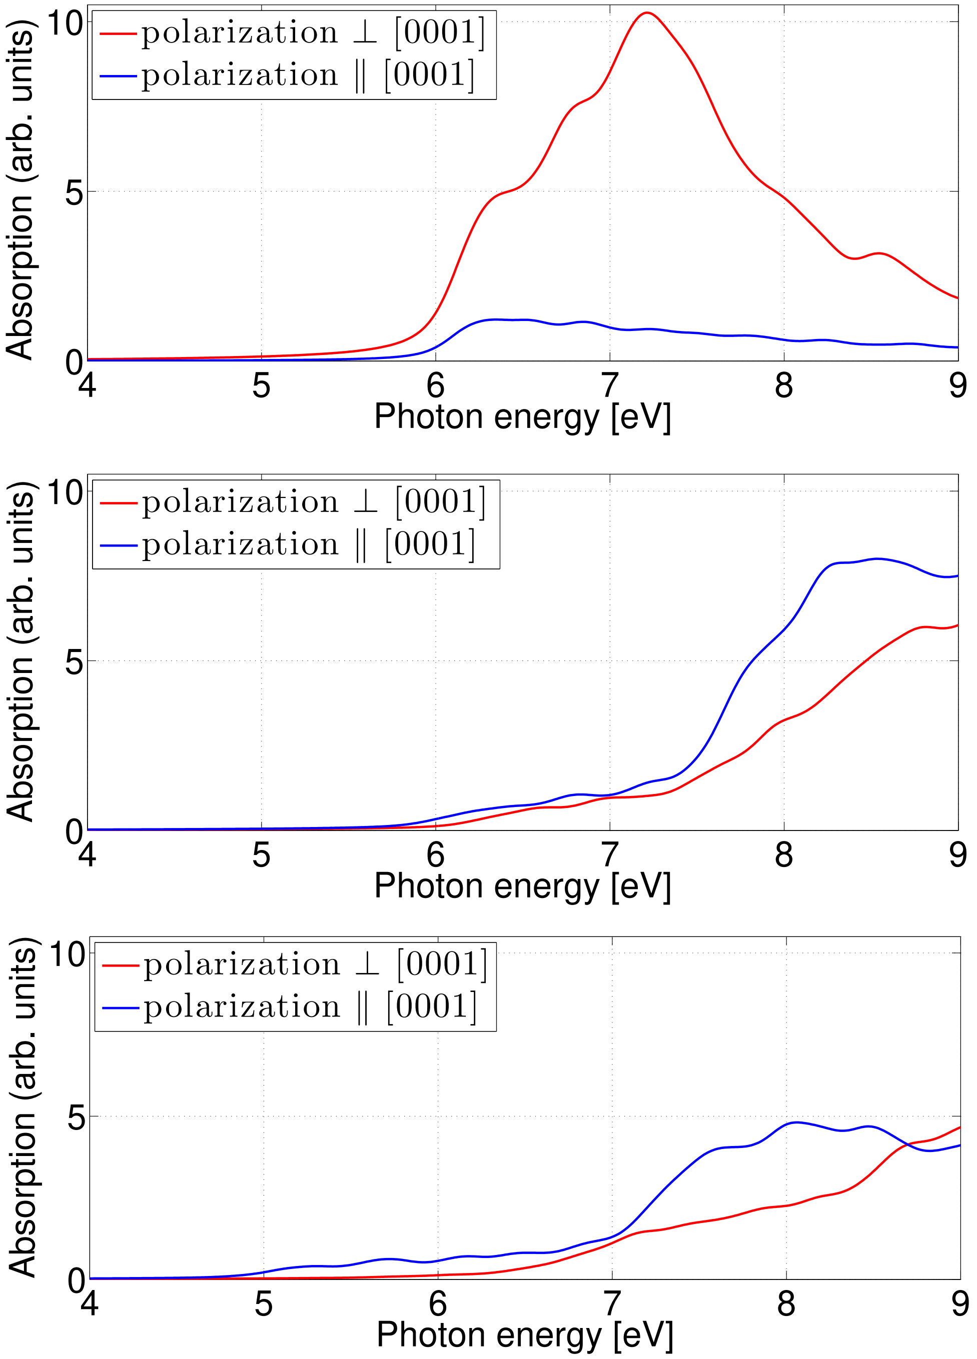


FIG. S7: (a) Optical absorption spectrum for light polarization perpendicular to [0001] (red line) and parallel to [0001] (blue line) of bulk: a) hBN, b) AlN wurtzite phase (wAlN), c) AlN hexagonal phase (hAlN). Spectra were obtained within the independent particle picture using hybrid DFT (HSE06) wavefunctions and eigenvalues. The Brillouin zone was sampled with the following k-point grids: 24x24x9 (hBN), 24x24x15 (wAlN) and 22x22x18 (hAlN).
